# Supplementary material for: Flow over an espresso cup: Inferring 3D velocity and pressure fields from tomographic background oriented schlieren videos via physics-informed neural networks
Source: arXiv:2103.02807 ancillary file (2021-03-09)
Supplement: Supplementary file 1 [file supplements.pdf]

# Supplementary materials

# Flow over an espresso cup: Inferring 3D velocity and pressure fields from tomographic background oriented schlieren videos via physics-informed neural networks

Shengze Cai[1], Zhicheng Wang[1], Frederik Fuest[2], Young Jin Jeon[2], Callum Gray[3], George Em Karniadakis[1]

[1]Division of Applied Mathematics, Brown University, Providence, RI, 02912, USA
[2]LaVision GmbH, Anna-Vandenhoeck-Ring 19, D-37081 Goettingen, Germany
[3]LaVision Inc., 211 W. Michigan Ave., Ypsilanti, MI 48197, USA

March 3, 2021

## 1 Quantifying the accuracy of PINN using synthetic data

Here, we evaluate the proposed PINN method using data from a direct numerical simulation. Specifically, a 2D natural convection simulation was performed to generate the temperature, velocity as well as pressure fields. Then, we apply PINNs to quantify the velocity and pressure fields from the temperature data. As the CFD simulation results can be used as reference, we can systematically evaluate the accuracy of the inferred fields.

### 1.1 2D problem setup

A 2D heat transfer problem of buoyancy-driven flow is numerically simulated using the spectral/$hp$ element method, which is implemented in the CFD solver NekTar. The simulation domain is defined as follows: $\Omega : [-0.015, 0.015] \times [0, 0.03]$ m. We assume that there is a heat source placed on the lower boundary: $x \in [-0.0076, 0.0076]$ m and $y = 0$, where the temperature is constant at $T_{hot} = 19.80$ K. Otherwise, the temperature is zero elsewhere on the bottom. For both temperature and velocity, periodic boundary conditions are used on the lateral boundaries, where $x = \pm 0.015$ m and the Neumann boundary condition is applied on the upper boundary, where $y = 0.03$ m. The environmental temperature is set as $T_\infty = 0$. This is a natural convection setup which is similar to the espresso cup experiment and the flow is driven only by the temperature difference between the source and the environment. The governing equations of this problem are given by the Boussinesq approximation of NS equations and the heat equation, where the physical properties are:

$$\begin{aligned}
&\alpha = 2.074 \times 10^{-5} \ \ \mathrm{m^2/s}, \quad \beta = 3.4 \times 10^{-3} \ \ 1/\mathrm{K}, \\
&\nu = 1.516 \times 10^{-5} \ \ \mathrm{m^2/s}, \quad \rho = 1.204 \ \ \mathrm{kg/m^3}, \quad g = 9.8 \ \ \mathrm{m/s^2}
\end{aligned} \tag{1.1}$$

By choosing the characteristic length and the characteristic velocity $L = 0.015$ m, $U = 0.1$ m/s, we have the non-dimensional parameters: Re $\approx 100$, Pe $\approx 71$, Ri $\approx 1.0$. The simulation has been carried out until both flow and temperature are well-developed. Then the temperature, velocity and pressure fields are collected with $\Delta t = 0.01$ s, resulting in a data set with 100 snapshots and 9950 data points per snapshot in space. Note that the data grid in this case depends on the element used in the simulation, while in practice, it corresponds to the resolution of the observed data (one data point refers to one pixel or one voxel). In addition, in order to investigate the sensitivity of the spatial resolution, we also generate image-like data, where the data is interpolated on a uniformly-distributed grid from CFD data. By using different grid scales, we can generate data with various resolutions, which are more consistent with the real experimental data.

We also note that in this synthetic assessment, the temperature, that is the only information used for PINNs training, is directly generated by CFD simulation. However, the temperature is generally reconstructed by analyzing the raw BOS images in real experiments (like the Tomo-BOS experiment in the main text). Considering a BOS image generation procedure, which models the optical system, the optical transfer function, *etc*, will make the problem more realistic and is worth investigating in the future to further validate the proposed method.

Here, we aim at inferring the velocity and pressure fields from the temperature data. Therefore, the temperature of all snapshots, generated artificially from CFD, is the only known information for the proposed algorithm, and no velocity or pressure boundary conditions are imposed anywhere. The simulated velocity and pressure are considered as the reference fields and will be used for validation of the PINNs results.

## 1.2 Evaluation metrics

To evaluate the performance of the proposed method, we define the relative $L_2$-norm error as

$$\epsilon_V = \| \hat{V} - V \|_2 \, / \, \| V \|_2 \times 100\%, \tag{1.2}$$

where $V$ denotes any quantity of the inferred outputs $(T, u, v, p)$; the hat represents the values estimated by PINNs, and the $L_2$-norm is computed over all the grid points. In addition, for the velocity estimation, we also compute the root mean square error (RMSE), which is a commonly-used metric in experimental fluid dynamics:

$$\text{RMSE} = \sqrt{\frac{1}{N}\sum_{i=1}^{N}[(\hat{u}-u)^2 + (\hat{v}-v)^2]}. \tag{1.3}$$

## 1.3 Comparison results

**Dimensional and dimensionless results.** We first demonstrate the results of PINNs with dimensional and non-dimensional setups. In the context of PINNs, the training data and the equations in residual network can be either dimensional or non-dimensional. However, for the dimensional setup, two additional procedures are employed in our implementation. First, a normalization step is applied to the outputs of $\mathcal{F}_{NN}$ before substituting them to the residuals, to make their values of the same order. Second, another normalization is used for the residuals to let them contribute equally to the loss function. In this test, we use neural networks with 10 hidden layers and 120 nodes per layer. The weighting coefficient in the loss function is 50. The networks are trained with Adam for 3500 epochs until convergence, with learning rate $6 \times 10^{-4}$.

The best results among ten independent training processes of PINNs are illustrated in Figure 1. The temperature, pressure, velocity vectors and streamlines at $t = 0.5$ s are shown. We find

that both setups of PINNs can provide velocity and pressure very accurately while fitting the temperature data. Moreover, two velocity profiles along $x = 0$ and $y = 0.015$ m are plotted in Figure 2, from which we can see that the PINN with dimensionless setup is slightly better than the PINN with dimensional setup, as the profiles are more consistent with the reference CFD results. The results can be evaluated quantitatively as well. The errors of both PINNs for one snapshot and for all 100 snapshots are given in Table 1.

Table 1: Validation using synthetic data: RMSE and relative $L_2$ errors. PINN* denotes the PINN with dimensionless setup

| | Errors at $t = 0.5$ s | | Average errors $t \in [0, 1)$ s | |
|---|---|---|---|---|
| | PINN | PINN* | PINN | PINN* |
| RMSE [m/s] | $8.5e{-}4$ | $6.8e{-}4$ | $8.6e{-}4$ | $7.0e{-}4$ |
| $\epsilon_T$ | 0.16% | 0.10% | 0.16% | 0.10 % |
| $\epsilon_u$ | 4.09% | 4.90% | 4.16% | 4.97% |
| $\epsilon_v$ | 5.73% | 3.16% | 5.85% | 3.32% |
| $\epsilon_p$ | 3.47 % | 2.72% | 3.67% | 2.82% |

In order to assess the influence of different factors on PINNs, we also perform a systematic study on the artificial data as we have the CFD result as a reference. In the following, the mean errors and the standard deviations of ten independent training processes are reported for each condition since the results may be affected by the random initialization of parameters. For clarity, we only perform the assessments on PINN with the dimensionless setup.

**Effect of weighting coefficient $\lambda$.** The weighting coefficient $\lambda$ plays an important role in adjusting the contributions of different terms (data mismatch and residual loss) in the loss function. In general, a large weight can accelerate the convergence since the temperature data can be regressed quickly, while it will weaken the contribution of the residuals and lead to data overfitting. This can be observed in Figure 3, where (a) shows the losses during PINN training and (b) shows the inference errors of five typical values of $\lambda$. As the losses illustrate, the weight is important in balancing the values of the two loss terms. In particular, while the minimal error of temperature is achieved when $\lambda = 1000$ (overfitting occurs), the best velocity result is obtained for $\lambda = 50 - 100$. Therefore, we recommend to choose a moderate value of $\lambda$ throughout the paper.

**Effect of neural network size.** The size of the neural network is represented by depth$\times$width, where depth denotes the number of hidden layers and width the number of neurons per layer. We apply various architectures for the dimensionless PINN. The resulting errors are shown in Figure 4. As we can see in the error plots of (a), small networks cannot approximate the solutions accurately. The errors decreases as the network size increases, and then remains nearly constant. We find that the best size for this 2D natural convection problem is the one with 10 hidden layers. In Figure 4(b), we demonstrate the absolute errors of velocity magnitude for two configurations, namely the network size $4 \times 50$ and $10 \times 100$, where we find that the large errors generally occur in the region where the temperature gradient is small (see the error of $4 \times 50$). However, this can be overcome when a larger neural network is used to approximate the solutions, as shown in the error contours of $10 \times 100$, where the error over the whole domain is small.

**Effect of temporal resolution.** The spatio-temporal resolution of the input temperature data is an important factor for PINNs. Instead of using 100 snapshots (i.e., time step $\Delta t = 0.01$ s) for training, now we use coarser data with multiple time steps. For example, if the data is sampled with $\Delta t = 0.10$ s, then the training dataset only contains 10 snapshots. The size of the neural network is $10 \times 100$. From the error plots in Figure 5, we can find that there is a transition

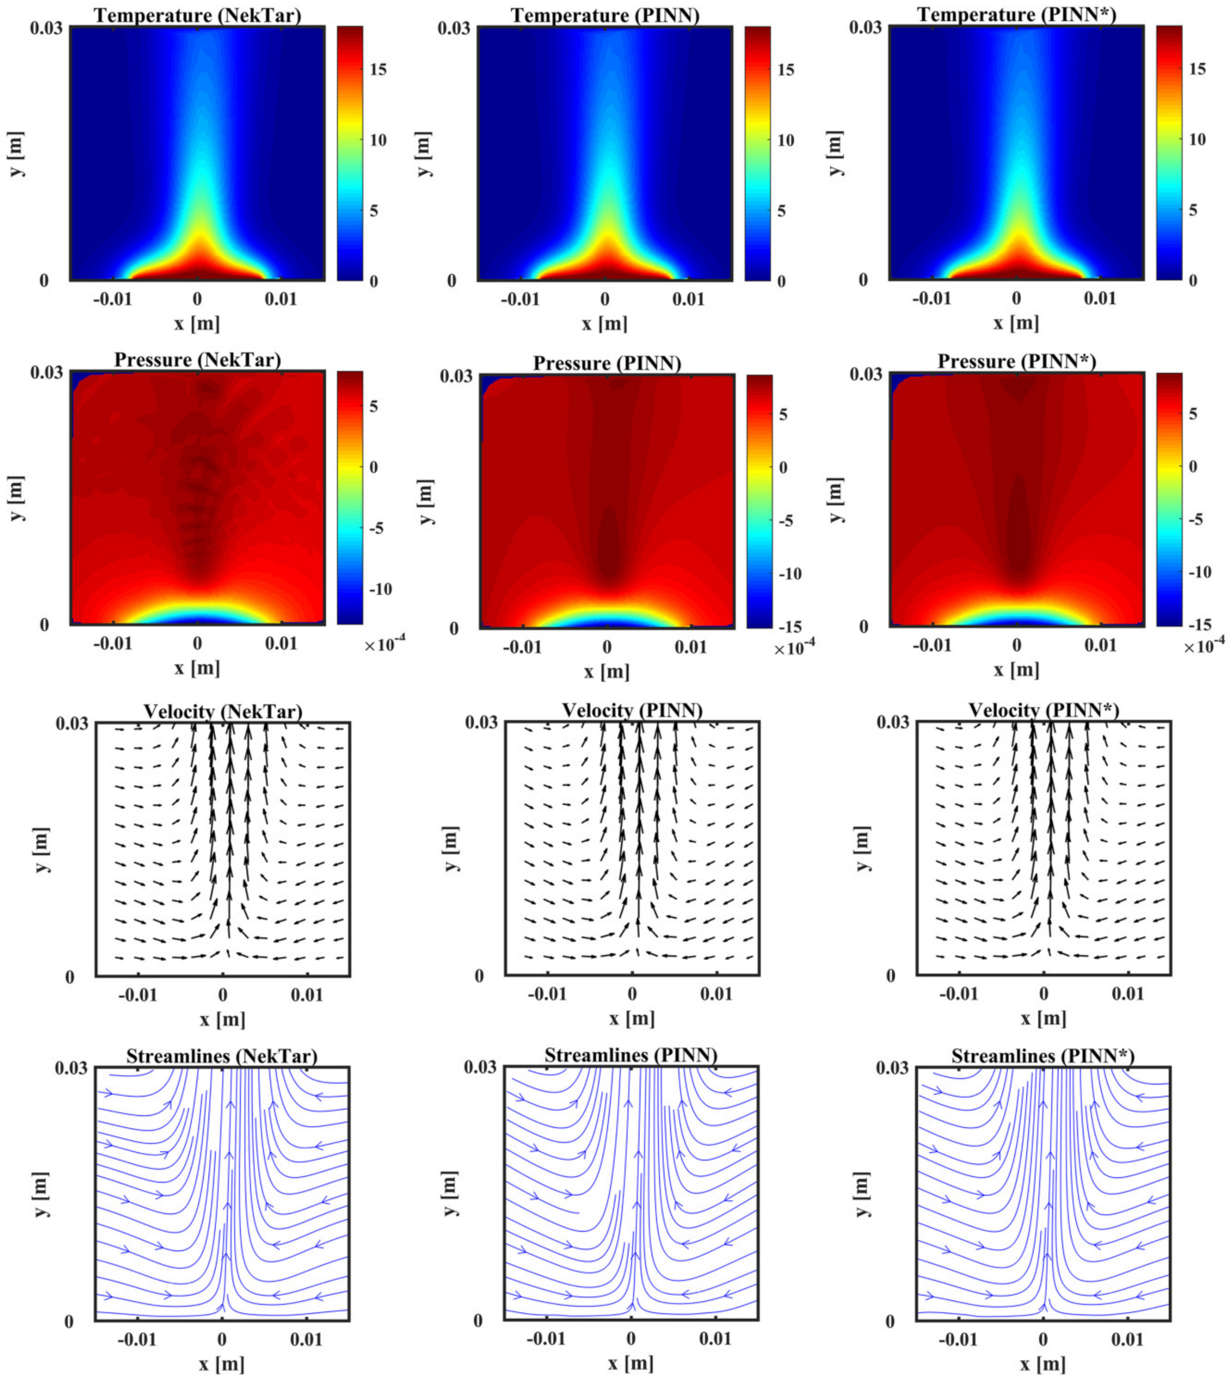


Figure 1: Validation using synthetic data: temperature, pressure, velocity vectors and streamlines of the natural convection problem at $t = 0.5$ s. First column: NekTar simulations, second column: results from PINN with dimensional setup, third column: results from PINN with dimensionless setup (denoted by PINN*). The $L_2$ errors and RMSE of dimensional PINN are $\epsilon_T = 0.16\%$, $\epsilon_p = 3.47\%$ and RMSE $= 8.5 \times 10^{-4}$ m/s, while those of non-dimensional PINN are $\epsilon_T = 0.10\%$, $\epsilon_p = 2.72\%$ and RMSE $= 6.8 \times 10^{-4}$ m/s.

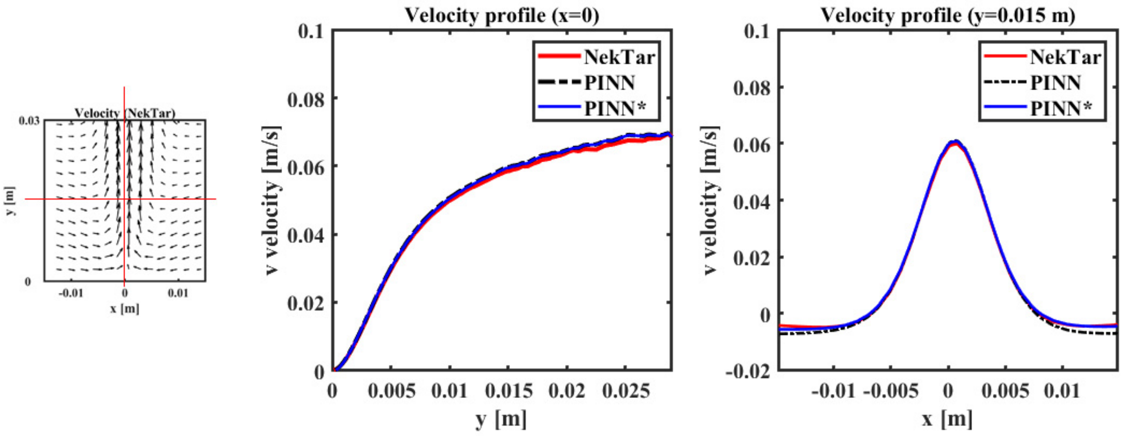


Figure 2: Validation using synthetic data: one-dimensional velocity profiles of the $v$-component at $t = 0.5$ s. Left: velocity profiles at $x = 0$, right: velocity profiles at $y = 0.015$ m. The black dot lines are the results from PINN with dimensional setup, while the blue lines are from PINN with dimensionless setup (denoted by PINN*).

point at $\Delta t = 0.10$ s, showing that the errors and the corresponding standard deviations increase dramatically when $\Delta t > 0.10$ s. For the data with $\Delta t = 0.1$ s, the maximum displacement between two snapshots is approximately 0.007 m, which corresponds to about 0.5 characteristic length of the flow. Note that although we use sparse data for training, the inference results are still evaluated by comparing with the CFD data with $\Delta t = 0.01$ s, because the trained network can infer the continuous velocity and pressure fields at any time instant. In other words, the errors presented here are computed over all 100 snapshots. The results of Figure 5(a) indicate that PINN is able to infer higher-resolution solutions ($\Delta t = 0.01$ s) with good accuracy based on the data which is not resolved very well. Moreover, the absolute errors of velocity magnitude for $\Delta t = 0.15$s and $\Delta t = 0.02$s are illustrated in Figure 5(b).

**Effect of spatial resolution.** Similar results can be found when we investigate the sensitivity of spatial resolution. As mentioned above, in this test we generate image-like data, where the data is interpolated on a uniformly-distributed grid from CFD data. By using different grid scales, we can generate data with various resolutions, as shown in Figure 6. Note that in the plots, the errors are computed by comparing with the ground-truth on the 128×128 grids. We find that using a coarse resolution of 24×24 grids allows us to have good estimations ($\epsilon_v \leq 10\%$). Here, the spatial domain is $0.03 \times 0.03$ m$^2$ and the characteristic length is $L = 0.015$ m. Therefore, the data with 24×24 grid points corresponds to a grid spacing of about 1.3 mm ($0.087L$). Moreover, the absolute errors of the velocity magnitude for $16 \times 16$ and $96 \times 96$ are illustrated in Figure 5(b), where we find the largest errors occur near the boundaries. The assessment of spatio-temporal resolution indicates that our method, which can reconstruct high-resolution fields from relatively sparse data, is promising in practice since higher spatio-temporal resolution of BOS images is generally more expensive.

**Effect of data noise.** In order to verify the robustness of the proposed method, we add artificial white noise to the temperature data. Specifically, we consider Gaussian noise $a \cdot \mathrm{Std}(T) \cdot \eta$, where $\eta$ is Gaussian noise with zero mean and unit variance. The noise level $a$ is defined by the ratio of noise magnitude to the standard deviation of the temperature data. The errors corresponding to various noise levels are presented in Figure 7. We can observe that the proposed algorithm is rather

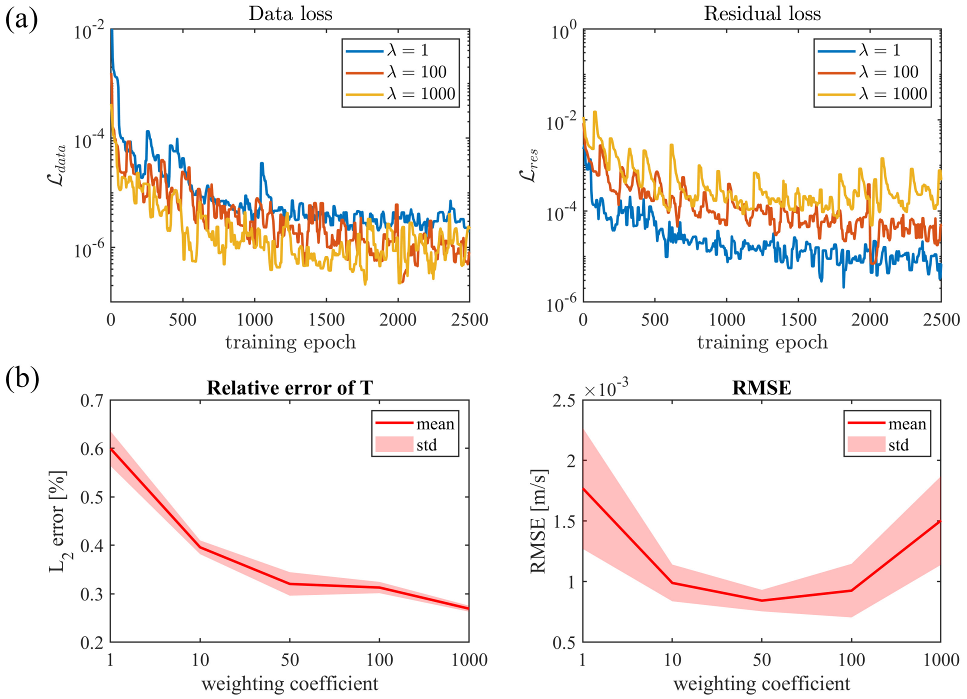


Figure 3: Effect of weighting coefficient $\lambda$: (a) data loss $L_{data}$ and residual loss $L_{res}$ with different $\lambda$; (b) $L_2$-norm error of temperature and the RMSE with respect to the weighting coefficient.

robust against the noise of training data. Even when the noise level $a$ is as high as 1.2, the errors of estimated velocity and pressure are about 2.5 times larger than the results without noise. The results indicate that the physical model encoded in the neural network has a strong regularization effect on the estimated fields.

**Computational cost.** The computational cost of training a PINN model is higher than the conventional velocimetry methods, such as cross-correlation, due to the required optimization process of a neural network with complex governing equations. The training time of PINNs, dependent on the size of neural network and the size of dataset, is summarized in Table 2 along with the corresponding errors. We find that processing the whole dataset with a large network results in a very high accuracy of the inference results, but it is relatively time-consuming. The efficiency of PINN training can be dramatically improved by reducing the network size or downsampling the dataset, which will not significantly affect the accuracy. We note that the application of multi-GPU training or transfer learning could boost the computational efficiency of the proposed method in the future.

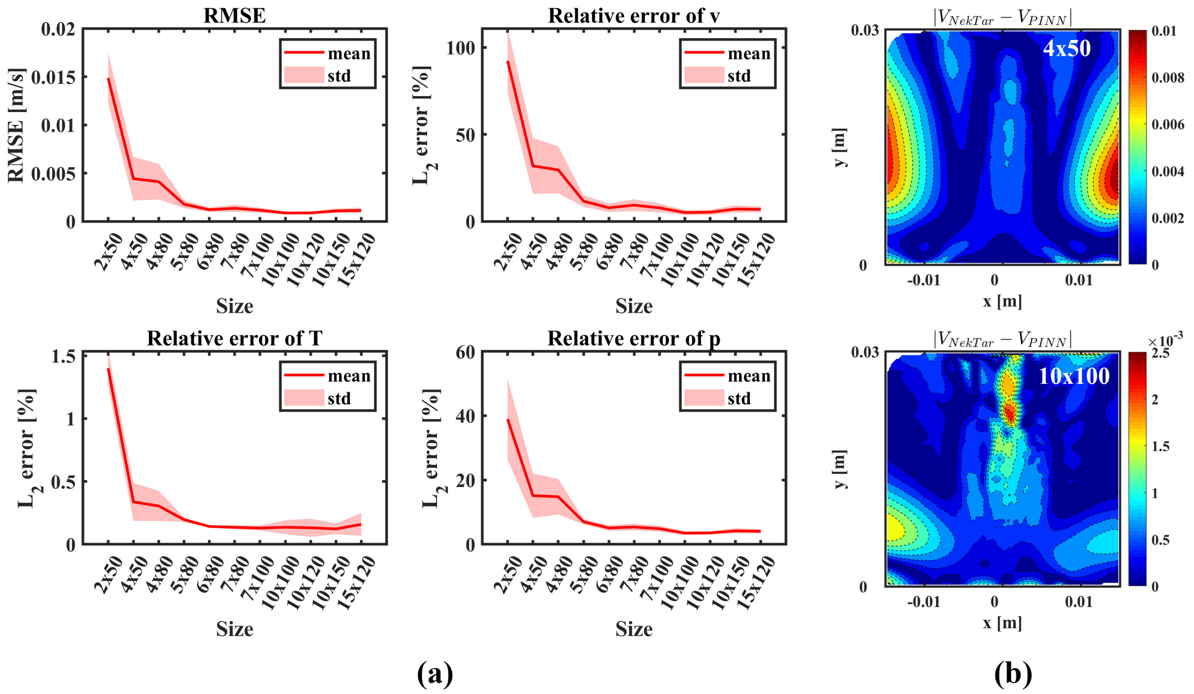


Figure 4: Effect of neural network size: (a) inference errors with various neural network sizes; (b) absolute errors of velocity magnitude (unit: m/s) under two configurations ($4 \times 50$ and $10 \times 100$). The RMSE as well as the $L_2$-norm errors of $v$-velocity, temperature and pressure are presented. The size of the neural network is represented by depth $\times$ width, where depth denotes the number of hidden layers and width the number of neurons per layer.

Table 2: Computational cost and errors of PINNs with respect to the size of neural network and the size of dataset. Note that the errors ($\epsilon_T$ and $\epsilon_v$) are computed over the full computational domain ($128 \times 128 \times 100$). The PINNs training is performed on a single Quadro RTX 6000 GPU.

| Spatial resolution | Number of frames | NN size | Time (hours) | $\epsilon_T$ (%) | $\epsilon_v$ (%) |
|---|---|---|---|---|---|
| $128 \times 128$ | 100 | $10 \times 100$ | 9.14 | 0.244 | 2.583 |
| $128 \times 128$ | 100 | $6 \times 80$ | 6.17 | 0.260 | 2.851 |
| $128 \times 128$ | 20 | $10 \times 100$ | 1.94 | 0.378 | 2.615 |
| $128 \times 128$ | 20 | $6 \times 80$ | 1.31 | 0.478 | 3.733 |
| $128 \times 128$ | 10 | $10 \times 100$ | 0.95 | 0.521 | 3.505 |
| $64 \times 64$ | 100 | $10 \times 100$ | 2.37 | 0.473 | 2.630 |
| $64 \times 64$ | 100 | $6 \times 80$ | 1.55 | 0.506 | 3.503 |
| $64 \times 64$ | 20 | $10 \times 100$ | 0.61 | 0.757 | 3.748 |
| $64 \times 64$ | 20 | $6 \times 80$ | 0.44 | 1.347 | 13.522 |

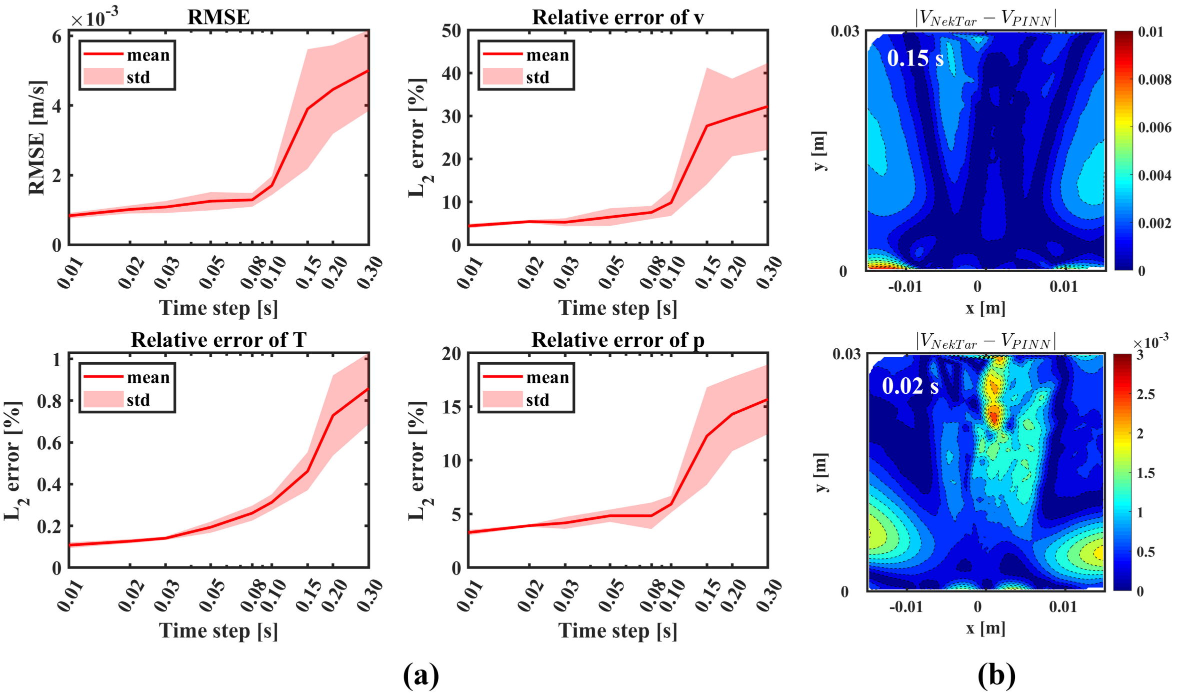


Figure 5: Effect of temporal resolution: (a) inference errors with various data sampling time steps; (b) absolute errors of velocity magnitude (unit: m/s) under two configurations ($\Delta t = 0.15$s and $\Delta t = 0.02$s). The RMSE as well as the $L_2$ errors of $v$-velocity, temperature and pressure are presented. For the data with $\Delta t = 0.1$ s, the maximum displacement between two snapshots is approximately 0.007 m, which corresponds to about 0.5 characteristic length of the flow.

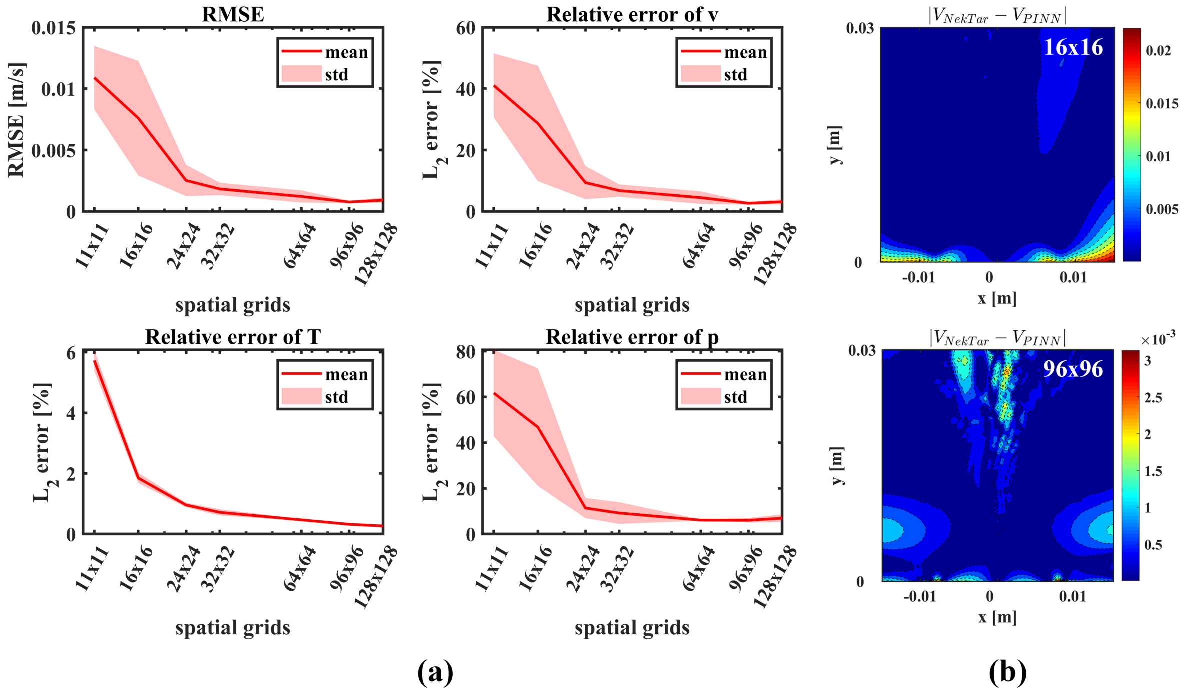


Figure 6: Effect of spatial resolution: (a) inference errors with various downsampling resolutions in space; (b) absolute errors of velocity magnitude (unit: m/s) under two configurations ($16 \times 16$ and $96 \times 96$). The RMSE as well as the $L_2$ errors of $v$-velocity, temperature and pressure are presented. The spatial domain is $0.03 \times 0.03$ m$^2$; the data with 24×24 points corresponds to a grid spacing of about 1.3 mm.

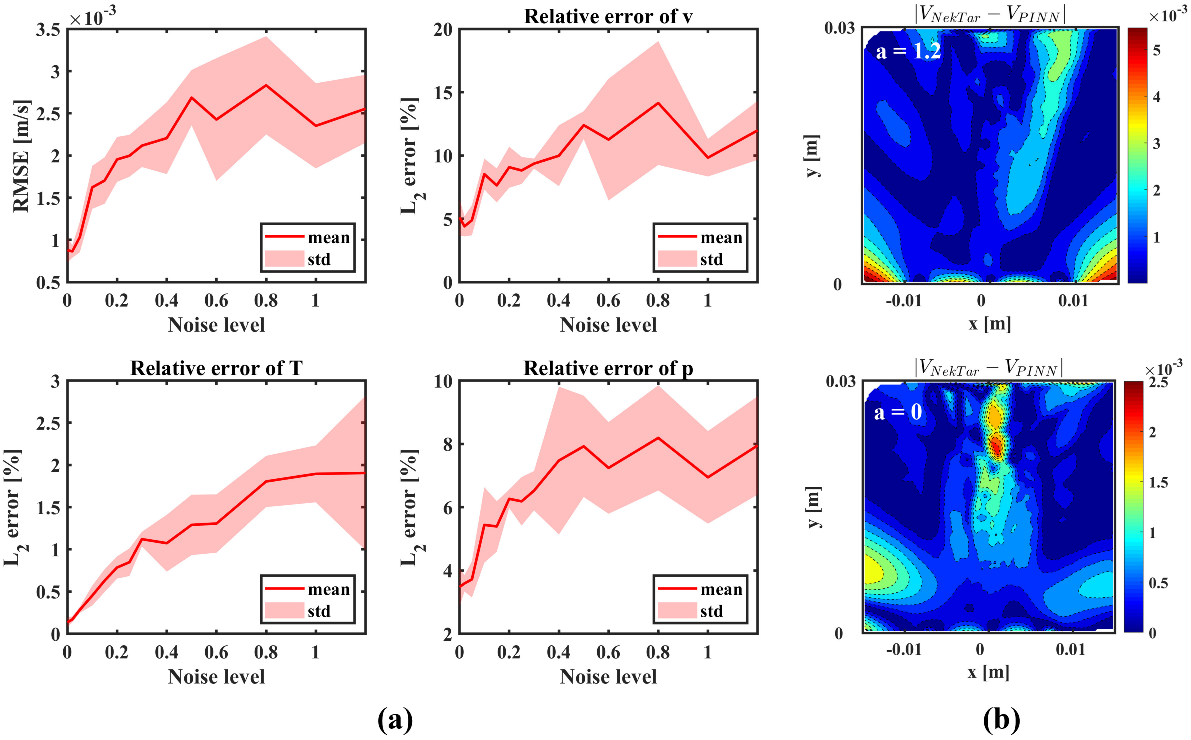


Figure 7: Effect of data noise: (a) inference errors with various noise levels of training data; (b) absolute errors of velocity magnitude (unit: m/s) under two configurations ($a = 1.2$ and $a = 0$). The RMSE as well as the $L_2$ errors of $v$-velocity, temperature and pressure are presented. The mean value and standard deviation are computed over ten independent training processes. The noise level $a$ is defined by the ratio of noise magnitude to the standard deviation of the original data.
